# Supplementary material for: Stable Prediction on Graphs with Agnostic Distribution Shift
Source: arXiv:2110.03865 source file (2021-10-08)
Supplement: Supplementary file 1 [file 6.Appendix.tex]

\section{Appendix}
\label{sec:appendix}

\begin{table}[htbp]
  \caption{Hyper-parameters}
  \label{tab:hyper}
  \small
  \begin{tabular}{l |r r r}
    \toprule
    Hyper-parameter        & OGB-Arxiv   & Citeseer    & Rec.   \\\midrule
    Batch size             & Full   &  Full  & 512     \\
    Training epochs         & 1,000 &  200  & 120 \\
    Initial learning rate  & 0.002  &  0.005  & 0.0001  \\
    Learning rate decay    & Linear &  None  & None \\
    Weight decay    & None &  5e-4  & None \\
    Adam $\epsilon$        & 1e-8   & 1e-8   & 1e-8   \\
    Adam $\beta_1$         & 0.9    &  0.9  & 0.9    \\
    Adam $\beta_2$         & 0.999  &  0.999  & 0.999  \\
    Number of layers       & 2      &  2  & 3      \\
    Hidden units per layer & 250     & 8   & 64     \\
    Dropout rate           & 0.75    &   0.6 & None    \\
    Input-drop rate           & 0.1    &  0.1  & 0.1    \\
    Edge-drop rate           & 0.1    &   None & None    \\
    \bottomrule
  \end{tabular}
  \normalsize
\end{table}

\subsection{Experiment Details}

\subsubsection{Hardware Configuration.} \  

The experiments are conducted on Linux servers equipped with an Intel(R) Xeon(R) Platinum 8163 CPU @ 2.50GHz, 330GB RAM and 8 NVIDIA Tesla V100-SXM2-16GB GPUs.

\subsubsection{Software Configuration.} \

Our framework is implemented in PyTorch \cite{NEURIPS2019_9015} with version 1.7.0, DGL \cite{Wang_Yu_Zheng_Gan_Gai_Ye_Li_Zhou_Huang_Ma_2019} with version 0.5.2, CUDA version 10.2, and Python 3.6.12. Code and datasets will be made publicly available.

\subsubsection{Detailed Hyper-parameters.}

The detailed hyper-parameters are listed in Table \ref{tab:hyper}.

\subsection{Implementation of Models}

\subsubsection{Generic SOTA GNNs} \

\vpara{GCN \cite{Kipf_Welling_2017}, GAT \cite{Velickovic_Cucurull_Casanova_Romero_Li_Bengio_2018}} We download the source code provided by the DGL Team \cite{Wang_Yu_Zheng_Gan_Gai_Ye_Li_Zhou_Huang_Ma_2019}. These implementations are tuned by the DGL Team especially for the OGB-Arxiv dataset. We set the hyper-parameters the same as described in Table \ref{tab:hyper}. Other hyper-parameters for each particular model are set as default in the source code.

Code: \url{https://github.com/dmlc/dgl/tree/master/examples/pytorch/ogb/ogbn-arxiv}

\vpara{SGC \cite{Wu_Souza_Zhang_Fifty_Yu_Weinberger_2019}} We implement SGC by directly replacing the graph convolution operator in the above GCN implementation with the SGConv provided by the DGL Team \cite{Wang_Yu_Zheng_Gan_Gai_Ye_Li_Zhou_Huang_Ma_2019}. All input parameters to construct the SGConv component stay the same as the GCNConv component.

\vpara{APPNP \cite{Bojchevski_Klicpera_Perozzi_Kapoor_Blais_Rzemberczki_Lukasik_Gnnemann_2020}} We implement APPNP by adding one more APPNP layer upon the output layer of GCN model. We set hyperparameters: $K=5$, teleport probability $\alpha=0.1$ with edge dropout rate $0.1$.

%\subsubsection{Generic SOTA GNNs for the Citeseer dataset} \

\subsubsection{SOTA GNNs that deal with selection bias} \

\vpara{GAT\_DVD} We download the authors’ official source code and change the hyper-parameter settings according to Table \ref{tab:hyper}.

Code: \url{https://openreview.net/forum?id=xboZWqM_ELA} (Supplementary Material).

\vpara{GNM} We download the authors’ official source code. Hyper-parameters are changed according to Table \ref{tab:hyper} and other model-specific hyper-parameters stay the same as default. This source code is designed for binary classifications. We make necessary modifications such as changing the number of classes to the corresponding number of each dataset.

Code: \url{https://github.com/mlzxzhou/keras-gnm}

\subsubsection{Graph Recommenders} \label{app:graphrec} \

\vpara{NGCF} We use a Pytorch-based implementation and use default hyper-parameters provided by the authors.

Code: \url{https://github.com/huangtinglin/NGCF-PyTorch}

\vpara{LightGCN} We use a Pytorch-based implementation and use default hyper-parameters provided by the authors.

Code: \url{https://github.com/gusye1234/LightGCN-PyTorch}

\vpara{Stable Graph Recommender} We build the proposed stable graph recommender based on NGCF. NGCF largely follows the standard GCN model. The proposed stable graph recommender propagates embeddings on the user-item bipartite graph as the following:
\begin{align}
&\alpha^e_{u i}=\text { sigmoid }\left(\mathbf{a}^{e}\left[\mathbf{e}_{u}^{0} \| \mathbf{e}_{i}^{0}\right]\right) \\
&\mathbf{e}_{u}^{(k+1)}=\sigma\left(\mathbf{W}_{1} \mathbf{e}_{u}^{(k)}+\sum_{i \in \mathcal{N}_{u}} \frac{\alpha^e_{u i}}{\sqrt{\left|\mathcal{N}_{u}\right|\left|\mathcal{N}_{i}\right|}}\left(\mathbf{W}_{1} \mathbf{e}_{i}^{(k)}+\mathbf{W}_{2}\left(\mathbf{e}_{i}^{(k)} \odot \mathbf{e}_{u}^{(k)}\right)\right)\right) \\
&\mathbf{e}_{i}^{(k+1)}=\sigma\left(\mathbf{W}_{1} \mathbf{e}_{i}^{(k)}+\sum_{u \in \mathcal{N}_{i}} \frac{\alpha^e_{u i}}{\sqrt{\left|\mathcal{N}_{u}\right|\left|\mathcal{N}_{i}\right|}}\left(\mathbf{W}_{1} \mathbf{e}_{u}^{(k)}+\mathbf{W}_{2}\left(\mathbf{e}_{u}^{(k)} \odot \mathbf{e}_{i}^{(k)}\right)\right)\right)
\end{align}
where $\mathbf{e}_{u}^{(k+1)}$ and $\mathbf{e}_{i}^{(k+1)}$ denote the updated user and item embedding after $k$ layers propagation. $\sigma$ denotes a certain nonlinear activation function and is $\operatorname{LeakyReLU}$ as NGCF. $\mathcal{N}_{u}$ denotes the set of interacted items for user $u$ and $\mathcal{N}_{i}$ denotes the set of interacted users for item $i$. $\mathbf{W}_{1}$ and $\mathbf{W}_{2}$ are learnable transformation matrices. $\alpha^e_{u i}$ denotes the importance of interaction $<u,i>$ for representing user $u$ and item $i$. We note that interactions that are consistently important across environments $\mathcal{E}$ are stable properties, as illustrated in Section \ref{sec:localstable}. We keep a global $\alpha^e_{u i}$ for layers due to its efficiency and do not compute weights per layer. We note that deep candidate generation models, which recall Top K items from a billion-scale item gallery are largely sensitive to model efficiency. For example, one of the contribution of LightGCN is to remove the nonlinearity $\sigma$ in NGCF and thus improving efficiency. We train the stable graph recommender as illustrated in Section \ref{sec:training}.

\subsection{Datasets}

\vpara{OGB-Arxiv \footnote{https://github.com/snap-stanford/ogb}} \ We obtain the OGB-Arxiv dataset directly from the Open Graph Benchmark team \cite{Hu_Fey_Zitnik_Dong_Ren_Liu_Catasta_Leskovec_2020}. We directly use the train/val/test split provided by them.

\vpara{Citeseer \footnote{https://github.com/dmlc/dgl/tree/master/python/dgl/data}} \ We obtain the Citeseer dataset from the Deep Graph Library team \cite{Wang_Yu_Zheng_Gan_Gai_Ye_Li_Zhou_Huang_Ma_2019}. Since the original training set will be rather small after biased selection, we combine 400 samples randomly selected from the original validation set and the original training set to construct the new training set. The remaining samples are used for validation.

\vpara{Recommendation Dataset} \label{app:detailrec} \ We collect a industrial dataset from one of the world-leading e-commerce platforms during the period of June 11th, 2020 to June 15th, 2020, when an annual product promotion festival is being celebrated. In such a period, the promotion strategies from online shop owners can be various and time-evolving. Therefore, inconsistencies between the users' clicks and their satisfactions naturally exist, leading to distribution shift from the collected data and the real-world testing environment. We select users and items that have interactions in all the five days, which means we do not consider the cold-start setting. We mainly consider click interactions, which is common setting for the deep candidate generation phase in recommendation. We further select users that have 200-300 interactions to ensure the quality of data. We split the interactions into several environments according to the day they happen, and the statistics are listed in Table \ref{tab:datadesc}. We use data samples in the first day for training and use the remaining for evaluation. We keep the gender and age attributes for users. For users that do not provide with these attributes, we use the value predicted by the e-commerce platform. There are 8 age sections in the dataset, including 1-18, 19-25, 26-30, 31-35, 36-40, 41-50, 51-60, and >=61. We group 1-18 and 19-25 into a holistic section and the remaining in to another section. This split results in approximately equally-sized sections.

The user-item bipartite graph consists of user nodes and items nodes, which are connected by whether there are interactions in between. Solely id feature is considered and transformed to dense vectors using a learnable embedding matrix, which is a common practice for deep candidate generation models \cite{He_Deng_Wang_Li_Zhang_Wang_2020,Wang_He_Wang_Feng_Chua_2019}. The embedding matrix is learned along with the graph recommenders.

\subsection{Evaluation}

\vpara{OGB-Arxiv} We use the evaluator provided by the official OGB Team \cite{Hu_Fey_Zitnik_Dong_Ren_Liu_Catasta_Leskovec_2020} use node prediction accuracy as the performance score.

\vpara{Citeseer} We use node prediction accuracy as the score.

\vpara{Recommendation} Since we mainly focus on the matching phase of recommendation, we use a widely used evaluation protocol, Normalized Discounted Cumulative Gain (NDCG), as the score. Compared to Recall and Hit Ratio, NDCG considers the positions of recommended items. NDCG can be formally written as:
	\begin{align}
		\text{DCG@N} &= \frac{1}{|\mathcal{U}|} \sum_{u \in \mathcal{U}} \sum_{r \in \hat{\mathcal{I}}_{u, N}} \frac{\mathbbm{1}(r \in \mathcal{I}_{u})}{\log _{2}\left(i_{r}+1\right)} \\
		\text{NDCG@N} &= \frac{ \text{DCG@N} }{\text{IDCG@N}}
	\end{align}
%\begin{align}
%\text{NDCG@N}=\frac{1}{Z} \frac{1}{|\mathcal{U}|} \sum_{u \in \mathcal{U}} \sum_{k=1}^{N} \frac{\delta\left(\hat{i}_{u, k} \in \mathcal{I}_{u}\right)}{\log _{2}(k+1)}
%\end{align}
where $\mathcal{U}$ is the set of users, N is the number of recommended items, and $\hat{i}_{u, k}$ indicates the $k$th item recommended for user $u$. $\mathbbm{1}$ denotes the indicator function. $\text{IDCG@N}$ denotes the ideal discounted cumulative gain and is the maximum possible value of $\text{DCG@N}$.

\subsection{Proof} \label{app:proof}
\begin{align*}
	&\frac{1}{2}\sum_{e, e^{\prime} \in \mathcal{E}} \left( \mathcal{L}^{e} - \mathcal{L}^{e'} \right)^{2} = \sum_{e=0}^{N-1}\sum_{e'=e+1}^{N} \left( \mathcal{L}^{e} - \mathcal{L}^{e'} \right)^{2} \\
	=&\sum_{e=1}^{N-1} \sum_{e'=e+1}^{N}\left(\mathcal{L}^{e}-\bar{\mathcal{L}}\right)^{2}+\sum_{e=1}^{N-1} \sum_{e'=e+1}^{N}\left(\mathcal{L}^{e'}-\bar{\mathcal{L}}\right)^{2} \\
	&-2 \sum_{e=1}^{N-1} \sum_{e'=e+1}^{N}\left(\mathcal{L}^{e}-\bar{\mathcal{L}}\right)\left(\mathcal{L}^{e'}-\bar{\mathcal{L}}\right) \\
	=&\sum_{e=1}^{N-1} \sum_{e'=e+1}^{N}\left(\mathcal{L}^{e}-\bar{\mathcal{L}}\right)^{2}+\sum_{e'=2}^{N} \sum_{e=1}^{e'-1}\left(\mathcal{L}^{e'}-\bar{\mathcal{L}}\right)^{2} \\
	&-\left(\sum_{e=1}^{N} \sum_{e'=1}^{N}\left(\mathcal{L}^{e}-\bar{\mathcal{L}}\right)\left(\mathcal{L}^{e'}-\bar{\mathcal{L}}\right)-\sum_{e=1}^{N}\left(\mathcal{L}^{e}-\bar{\mathcal{L}}\right)^{2}\right) \\
	=&\sum_{e=1}^{N-1}(N-e)\left(\mathcal{L}^{e}-\bar{\mathcal{L}}\right)^{2}+\sum_{e'=2}^{N}(e'-1)\left(\mathcal{L}^{e'}-\bar{\mathcal{L}}\right)^{2} \\
	&-\left(\sum_{e=1}^{N}\left(\mathcal{L}^{e}-\bar{\mathcal{L}}\right) \sum_{e'=1}^{N}\left(\mathcal{L}^{e'}-\bar{\mathcal{L}}\right)-\sum_{e=1}^{N}\left(\mathcal{L}^{e}-\bar{\mathcal{L}}\right)^{2}\right) \\
	=&\left((N-1)\left(\mathcal{L}^{1}-\bar{\mathcal{L}}\right)^{2}+\sum_{e=2}^{N-1}(N-e)\left(\mathcal{L}^{e}-\bar{\mathcal{L}}\right)^{2}\right) \\
	&+\left(\sum_{e'=2}^{N-1}(e'-1)\left(\mathcal{L}^{e'}-\bar{\mathcal{L}}\right)^{2}+(N-1)\left(\mathcal{L}^{N}-\bar{\mathcal{L}}\right)^2\right) \\
	&-\left(0-\sum_{e=1}^{N}\left(\mathcal{L}^{e}-\bar{\mathcal{L}}\right)^{2}\right) \\
	=&(N-1)\left(\mathcal{L}^{1}-\bar{\mathcal{L}}\right)^{2}+\sum_{e=2}^{N-1}(N-1)\left(\mathcal{L}^{e}-\bar{\mathcal{L}}\right)^{2}+ \\
	&(N-1)\left(\mathcal{L}^{N}-\bar{\mathcal{L}}\right)^{2}+\sum_{e=1}^{N}\left(\mathcal{L}^{e}-\bar{\mathcal{L}}\right)^{2} \\
	=&N \sum_{e=1}^{N}\left(\mathcal{L}^{e}-\bar{\mathcal{L}}\right)^{2} 
\end{align*}
where $\bar{\mathcal{L}}$ denotes the average loss of all environments.
